# Supplementary material for: Head-wise Adaptive Rotary Positional Encoding for Fine-Grained Image Generation
Source: arXiv:2510.10489 source file (2026-03-12)
Supplement: Supplementary file 1 [file X_suppl.tex]

\clearpage
\setcounter{page}{1}
\maketitlesupplementary

\section{Additional Qualitative Results}
We provide supplementary visual comparisons to illustrate the empirical effects of HARoPE:
Figure~\ref{fig:flux_compare_result} shows qualitative comparisons on GenEval prompts using FLUX-dev with RoPE vs. HARoPE, highlighting improvements in spatial relations, color fidelity, and object counts. 
Figure~\ref{fig:mmdit_coco_vis} demonstrates text-to-image examples on MS-COCO dataset using SD3-medium, comparing APE (Absolute Position Embedding) baselines and HARoPE.
The results illustrate gains in fidelity and compositional consistency. 
Figure~\ref{fig:multi_vs_single} visualizes HARoPE with and without head-wise specialization in FLUX.

\begin{figure*}
\centering
\includegraphics[width=1.0\textwidth]{picture/flux_compare_v3.pdf}
\caption{Qualitative Comparison on the GenEval Benchmark, evaluating FLUX-dev models with RoPE and HARoPE positional embeddings.}
\label{fig:flux_compare_result}
\end{figure*}

\begin{figure*}
\centering
\includegraphics[width=1.0\textwidth]{picture/mmdit_coco.pdf}
\caption{Text-to-image generation results trained on MS-COCO dataset. evaluating SD3-medium models with RoPE and HARoPE positional embeddings.}
\label{fig:mmdit_coco_vis}
\end{figure*}

\begin{figure*}
\centering
\includegraphics[width=1.0\textwidth]{picture/head_compare_new.pdf}
\caption{Visualization comparison of HARoPE with and without head-wise specialization, training and tested using Flux-dev on the text-to-image generation task.}
\label{fig:multi_vs_single}
\end{figure*}
